# Supplementary material for: Temporal Regular Path Queries
Source: arXiv:2107.01241 source file (2022-03-09)
Supplement: Supplementary file 1 [file appendix.tex]

\section{Proofs of Theorem \ref{th:main-summary}}
\label{sec-app-proofs}
